# Supplementary material for: IndiVec: An Exploration of Leveraging Large Language Models for Media Bias Detection with Fine-Grained Bias Indicators
Source: arXiv:2402.00345 source file (2024-02-01)
Supplement: Supplementary file 2 [file appendix_dataset_examples.tex]

\begin{table*}[t]
\setlength{\tabcolsep}{1mm}\small
\begin{center}
\resizebox{\linewidth}{!}{
\begin{tabular}{p{2.5cm}|p{9cm}|p{3.5cm}}
\toprule[1.0pt]

\textbf{Dataset} & \textbf{Examples} & \textbf{Remark} \\

\midrule[0.5pt]
\multirow{6}{\linewidth}{\textbf{FlipBias} \cite{chen-etal-2018-learning}}
 & Pair 1: 
 & \multirow{6}{\linewidth}{Only titles are given here, paired, article-level}\\
&Left: John McCain urges republicans not to filibuster gun control. 
 & \\
 & Right: White House looks to salvage gun-control legislation.& \\
  \cmidrule(lr){2-2}
 & Pair 2:  & \\
 & Left: Obama accepts nomination, says his plan leads to a “better place”. & \\
 & Right: Lackluster Obama: change is hard, give me more time. & \\
\midrule[0.5pt]
\multirow{3}{\linewidth}{\textbf{BASIL} \cite{fan2019plain}} & Biased: “Trump says he wants to run the nation like he’s run his business,” Mr. Bloomberg said on Wednesday.& \multirow{3}{\linewidth}{Paired, sentence-level}\\
& Non-biased: “But Trump’s business plan is a disaster in the making.”& \\
\midrule[0.5pt]
\multirow{6}{\linewidth}{\textbf{BABE} \cite{spinde2022neural}} &Biased: "We have one beautiful law," Trump recently said in his characteristically bizarre syntax and diction, repeating the word "beautiful." & \multirow{6}{\linewidth}{Non-paired, sentence-level}\\
&Non-biased: Orange Is the New Black star Yael Stone is renouncing her U S green card to return to her native Australia in order to fight climate change & \\
\midrule[0.5pt]
\multirow{6}{\linewidth}{\textbf{MFC} (V2)} \cite{card2015media} & Baised: BUSH WAIT ON GAY MARRIAGE BAN WASHINGTON President Bush stopped short yesterday of backing a constitutional amendment banning same sex marriages ... ... & \multirow{6}{\linewidth}{Non-paired, article-level} \\
& Non-biased: BECKNER REOPENS BENEFITS DEBATE Kevin Beckner Hillsborough County s first openly gay commissioner said he didn t run for office to promote a gay agenda But a little more than two months after ... ... & \\
\bottomrule[1.0pt]
\end{tabular}
}
\end{center}
\vskip -1em
\caption{\label{tab:appendix_dataset} Some Examples from FlipBias, BASIL, BABE, and MFC Datasets.
}
\vskip -1em
\end{table*}
